# Supplementary material for: Which Invariance Should We Transfer? A Causal Minimax Learning Approach
Source: arXiv:2107.01876 source file (2023-05-30)
Supplement: Supplementary file 1 [file related_works.tex]

\section{Related works}

\textbf{Causality-based domain generalization.} There are emerging works that consider the domain generalization problem from a causal perspective. One line of works \cite{arjovsky2019invariant, xie2020risk, muller2020learning,liu2021heterogeneous,ahuja2021invariance} promoted invariance as a key surrogate feature of causation where the causal graph is more of a motivation. Another line of works \cite{ilse2020diva, mahajan2020domain, lu2021nonlinear,mitrovic2021representation} considered domain generalization for unstructured data using specifically designed causal graphs to incorporate priors for the distributional shift, in which the causal features were modeled as latent variables to be inferred for robust prediction. 

The works most relevant to us pursued robust transfer by making invariance assumptions regarding causal mechanisms \cite{peters2016causal,buhlmann2020invariance,rojas2018invariant, subbaswamy2019preventing,subbaswamy2020spec}. Specifically, the \cite{peters2016causal,buhlmann2020invariance} assumed the causal mechanism that generated $Y$ from its parents was invariant; hence they only used the parental features for transfer. The \cite{rojas2018invariant} extended the invariance assumption and was able to use covariates beyond $\mathbf{Pa}(Y)$. The \cite{subbaswamy2019preventing, subbaswamy2020spec} considered a selection diagram framework, where mutable variables were children of the selection variable and had unstable causal mechanisms across environments. They then proposed to remove the unstable mechanisms by intervening on the mutable variables and obtained a set of stable predictors. To identify the optimal $S^* \subseteq S$, they first shown the whole stable set is optimal under the degeneration condition. For more general cases, they simply searched over all subsets in $S$ and took the one with minimal validation loss. However, their analysis is far from satisfactory, as the degeneration condition is hard to test and the subset selected via validation loss may not be optimal. \textbf{In contrast}, we provide a testable graphical condition and a comprehensive minimax analysis that guarantees the optimality of the selected subset. Further, to efficiently search for the optimal subset, we define an equivalence relation. We theoretically show its advantage over the exhaustive search adopted by \cite{subbaswamy2019preventing}.

\textbf{Optimization-based domain generalization.} Recently, there are works that view domain generalization as an optimization problem. These methods directly formulate the objective of out-of-distribution generalization and conduct optimization for robustness. For example, Distributional Robust Optimization (DRO) \cite{sinha2018certifiable} constrained the distance between training and deployment distributions with f-divergence or Wasserstein distance and optimized the minimax objective. One of its popular extensions, GroupDRO \cite{sagawa2019distributionally}, provided extra regularization (\emph{e.g.}, weight-decay or early stop) and allowed DRO models to achieve better performances in large neural networks. 

However, these methods heavily rely on data-driven optimization and lack analysis of the source of distributional shifts. For this reason, they have to constrain the distributional shifts to a limited extent, so as to achieve optimization convenience. Such a limitation affects their ability to generalize to broader distribution families and limits their applications in the real world. \textbf{In contrast}, we consider the domain generalization from a causal perspective. Benefiting from the causal interpretation, our method can attribute the distributional shifts to the unstable causal mechanisms of $\mathbf{X}_M$ and achieve minimax optimum even when the distribution shifts arbitrarily.

\textbf{Causal discovery in heterogeneous data.} Our work benefits from the recent progress in heterogeneous causal discovery \cite{ghassami2018multi,huang2019specific,mooij2020joint,huang2020causal}, a field that seeks to learn causal graphs with data from multiple environments. The objective of heterogeneous causal discovery is to recover as many as causal structures, in order to reveal the relations among variables. \textbf{In contrast}, we are only interested in causal structures that aid the minimax analysis and robust subset selection.
